# Supplementary material for: InSe: a two-dimensional material with strong interlayer coupling
Source: arXiv:1803.09919 source file (2018-03-27)
Supplement: Supplementary file 1 [file SI.pdf]

# Supporting Information

# InSe: a two-dimensional material with strong interlayer coupling

*Yuanhui Sun,*[a] *Shulin Luo,*[a] *Xin-Gang Zhao,*[a] *Koushik Biswas,*[b] *Song-Lin Li,**[c] *and Lijun Zhang**[a,d]

[a] Key Laboratory of Automobile Materials of MOE and College of Materials Science and Engineering, Jilin University, Changchun 130012, China

[b] Department of Chemistry and Physics, Arkansas State University, AR 72467, USA

[c] National Laboratory of Solid State Microstructures, School of Electronic Science and Engineering and Collaborative Innovation Center of Advanced Microstructures, Nanjing University, Nanjing 210023, China

[d] State Key Laboratory of Superhard Materials, Jilin University, Changchun 130012, China

**Corresponding Author**

*sli@nju.edu.cn
*lijun_zhang@jlu.edu.cn

**Table S1** The calculated lattice parameters with optB86b-vdW and optB88-vdW functionals for bulk β-InSe and γ-InSe. The selected functional is emphasized with purple background.

| | Bulk β-InSe | | | Bulk γ-InSe | | |
|---|---|---|---|---|---|---|
| Functional | B86b-vdW | B88-vdW | Exp.[1] | B86b-vdW | B88-vdW | Exp.[2,3] |
| a | 4.054 | 4.092 | 4.05 | 4.062 | 4.099 | 4.002 |
| b | 4.054 | 4.092 | 4.05 | 4.062 | 4.099 | 4.002 |
| c | 16.929 | 16.998 | 16.93 | 25.151 | 25.189 | 24.961 |

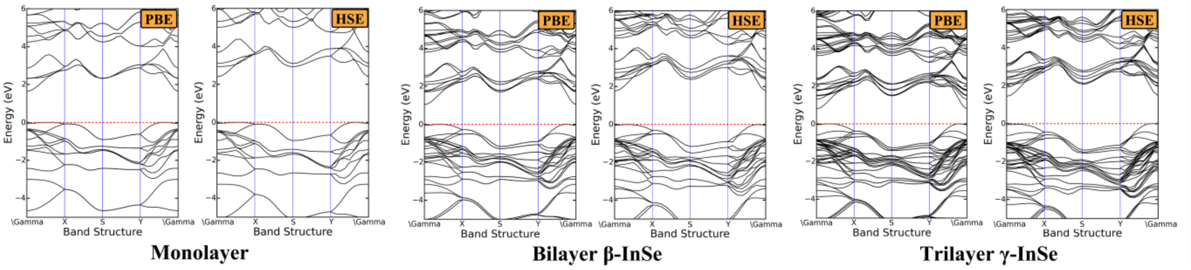


**Fig. S1** The calculated PBE and HSE06 band structures for monolayer, bilayer β-InSe, and trilayer γ-InSe, respectively.

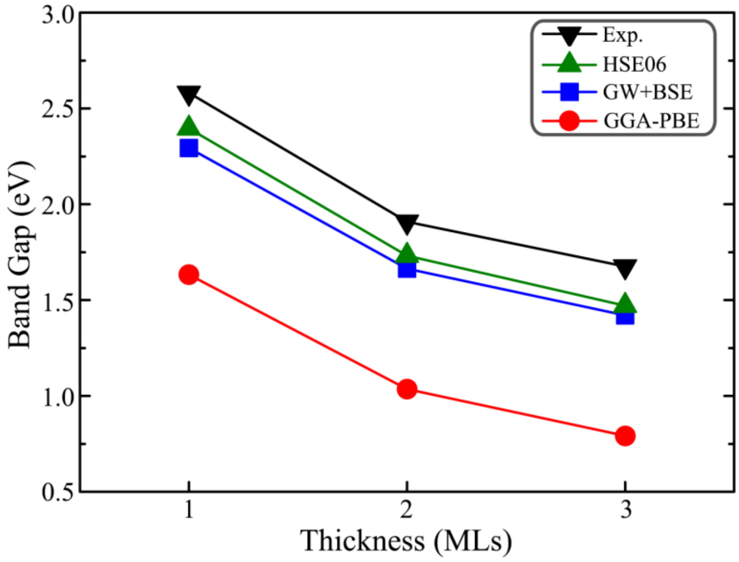


**Fig. S2** Evolution of electronic band gaps with varying thickness from monolayer to trilayer γ-InSe as obtained from experiment and different theoretical approaches.

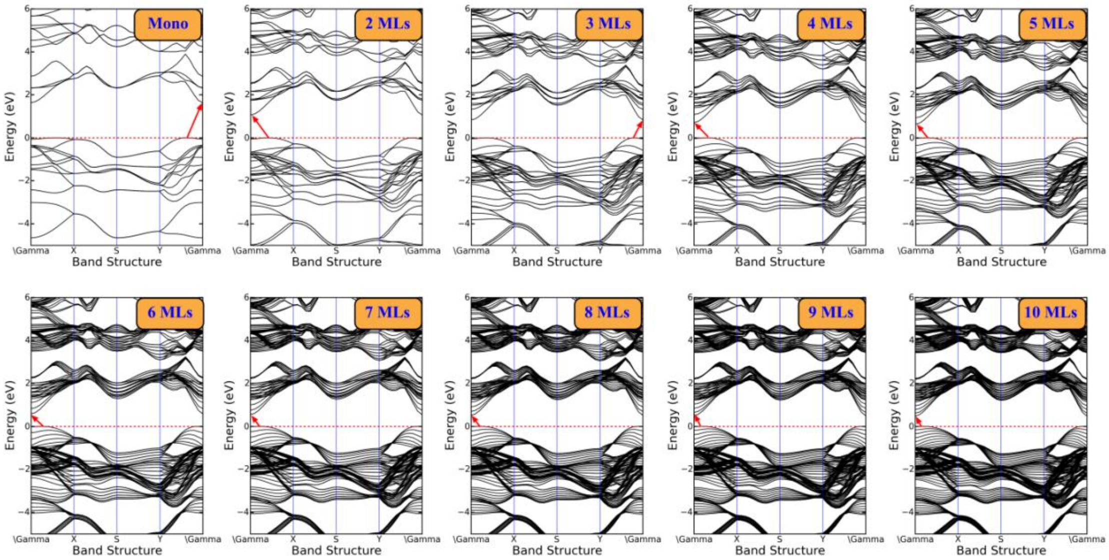


**Fig. S3** The calculated PBE band structures of β-InSe from $n$ = 1 to $n$ = 10-MLs. The arrows point the indirect gap positions.

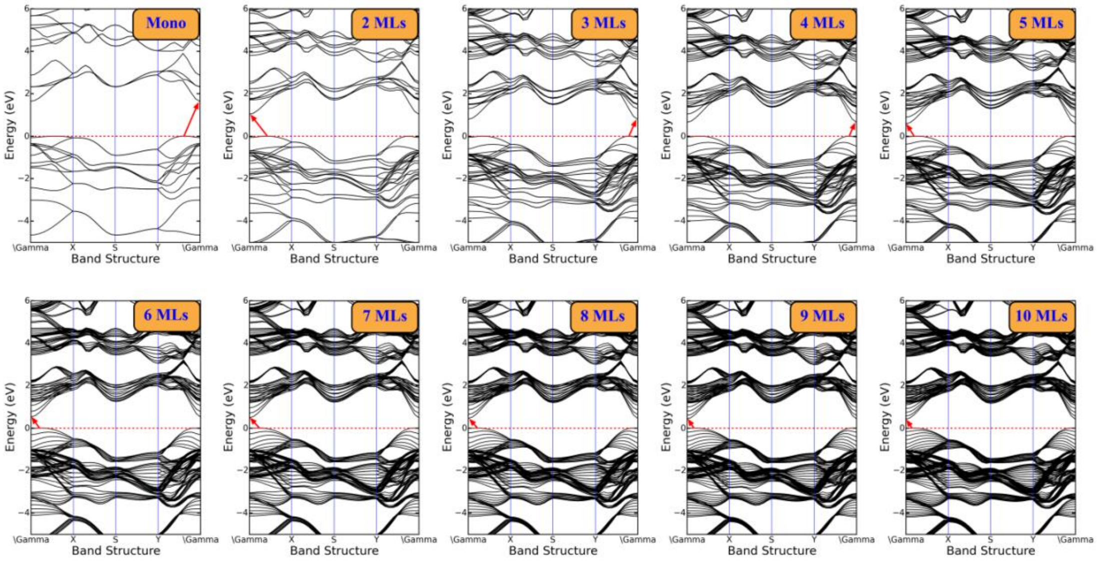


**Fig. S4** The calculated PBE band structures of γ-InSe from $n$ = 1 to $n$ = 10-MLs. The arrows point the indirect gap positions.

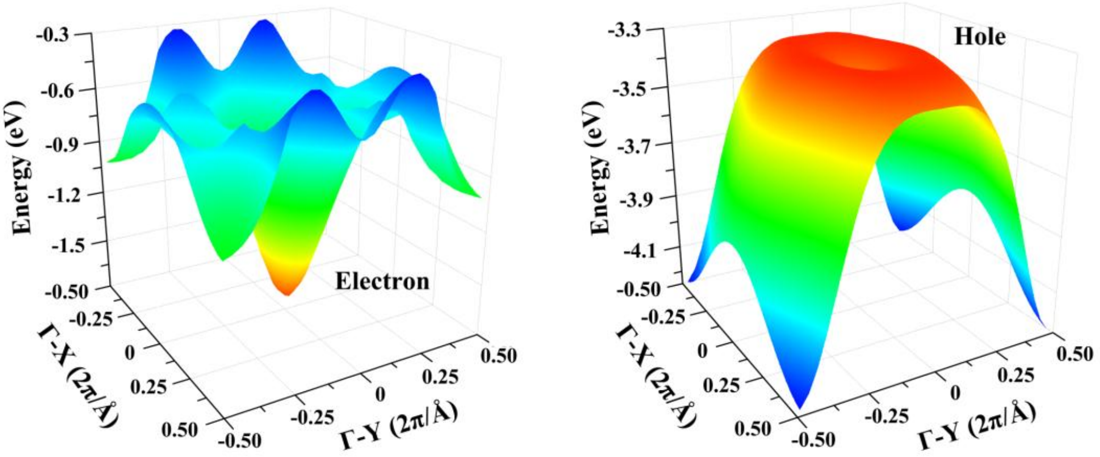


**Fig. S5** Contours of the lowest CB and the highest VB of monolayer InSe at the 2D plane of Brillouin zone.

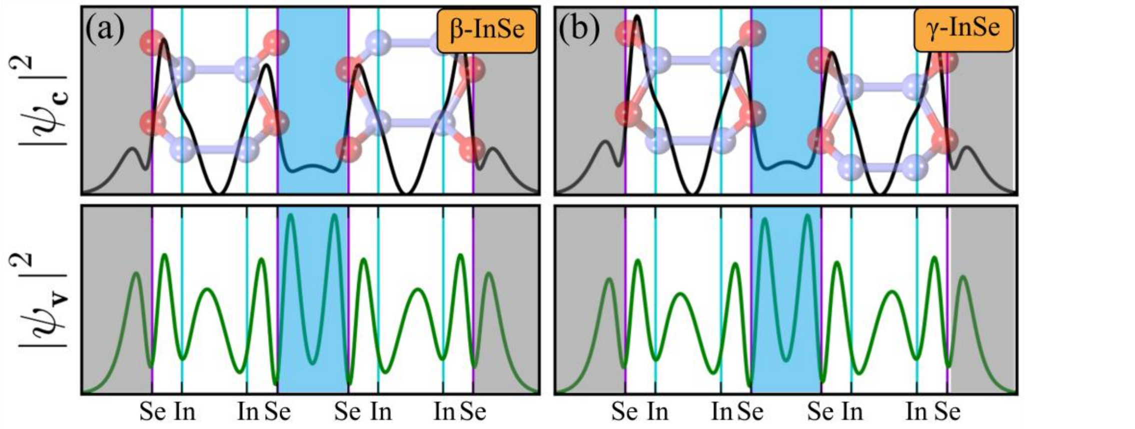


**Fig. S6** Planar-averaged squared magnitude of wave functions of the CBM and VBM states of bilayer (a) β-InSe and (b) γ-InSe, respectively. The dodgerblue and grey parts represent interlayer and vacuum regions, respectively.

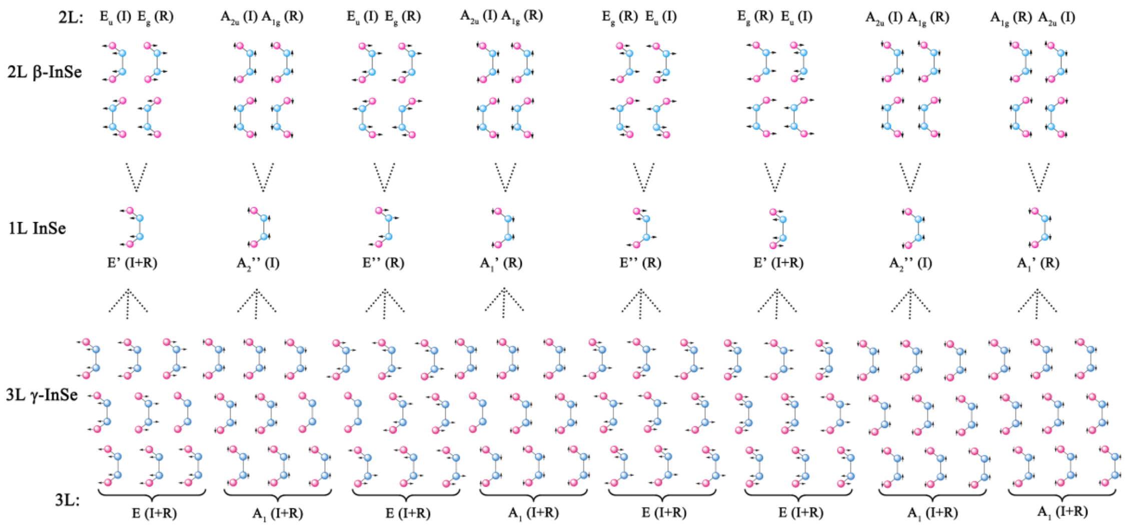


**Fig. S7** Vibration modes, symmetry representation, and optical activities (Raman: R; Infrared: I) of the phonon modes for monolayer, bilayer β-InSe, and trilayer γ-InSe, respectively.

**Table S2** The effective mass, deformational potential, 2D elastic modulus and the carrier mobility along x and y direction for β-InSe from $n$ = 1 to $n$ = to 10-MLs.

| **β-InSe** | **Carrier type** | **$m_x$ ($m_0$) Γ-X** | **$m_y$ ($m_0$) Γ-Y** | **$E_{1x}$ (eV)** | **$E_{1y}$ (eV)** | **$C_{x\_2D}$ (N/m)** | **$C_{y\_2D}$ (N/m)** | **$\mu_{x\_2D}$ ($cm^2V^{-1}s^{-1}$)** | **$\mu_{y\_2D}$ ($cm^2V^{-1}s^{-1}$)** |
|---|---|---|---|---|---|---|---|---|---|
| 1 layer | Electron | 0.20 | 0.23 | 5.70 | 5.76 | 52.35 | 52.89 | 801.09 | 689.20 |
| | Hole | 12.28 | 2.72 | 2.66 | 2.28 | 52.35 | 52.89 | 2.22 | 13.80 |
| 2 layers | Electron | 0.17 | 0.20 | 5.37 | 2.78 | 100.57 | 100.18 | 2372.77 | 7496.29 |
| 3 layers | Electron | 0.16 | 0.19 | 5.22 | 5.36 | 153.76 | 153.72 | 4313.90 | 3444.57 |
| 4 layers | Electron | 0.15 | 0.18 | 5.67 | 5.95 | 201.33 | 204.14 | 5418.69 | 4157.81 |
| 5 layers | Electron | 0.15 | 0.18 | 5.34 | 5.43 | 254.96 | 255.43 | 7736.44 | 6246.58 |
| 6 layers | Electron | 0.15 | 0.17 | 5.45 | 5.60 | 308.76 | 308.43 | 9255.32 | 7726.56 |
| 7 layers | Electron | 0.14 | 0.17 | 5.28 | 5.53 | 356.39 | 357.65 | 12623.09 | 9510.32 |
| 8 layers | Electron | 0.14 | 0.17 | 5.04 | 4.98 | 410.67 | 411.65 | 15963.94 | 13497.60 |
| 9 layers | Electron | 0.14 | 0.17 | 4.64 | 5.13 | 458.97 | 463.15 | 21050.21 | 14311.14 |
| 10 layers | Electron | 0.14 | 0.17 | 4.32 | 4.64 | 511.17 | 514.72 | 27046.19 | 19441.17 |

**Table S3** The effective mass, deformational potential, 2D elastic modulus and the carrier mobility along x and y direction for γ-InSe from $n$ = 1 to $n$ = to 10-MLs.

| **γ-InSe** | **Carrier type** | **$m_x$ ($m_0$) Γ-X** | **$m_y$ ($m_0$) Γ-Y** | **$E_{1x}$ (eV)** | **$E_{1y}$ (eV)** | **$C_{x\_2D}$ (N/m)** | **$C_{y\_2D}$ (N/m)** | **$\mu_{x\_2D}$ ($cm^2V^{-1}s^{-1}$)** | **$\mu_{y\_2D}$ ($cm^2V^{-1}s^{-1}$)** |
|---|---|---|---|---|---|---|---|---|---|
| 1 layer | Electron | 0.20 | 0.23 | 5.70 | 5.76 | 52.35 | 52.89 | 801.09 | 689.20 |
| | Hole | 12.28 | 2.72 | 2.66 | 2.28 | 52.35 | 52.89 | 2.22 | 13.80 |
| 2 layers | Electron | 0.17 | 0.19 | 5.34 | 5.37 | 100.56 | 100.08 | 2461.60 | 2167.55 |
| 3 layers | Electron | 0.16 | 0.18 | 3.93 | 4.94 | 151.29 | 155.50 | 7693.67 | 4448.69 |
| 4 layers | Electron | 0.15 | 0.18 | 5.10 | 5.15 | 205.81 | 202.75 | 6846.64 | 5512.10 |
| 5 layers | Electron | 0.15 | 0.17 | 5.30 | 5.44 | 255.64 | 255.36 | 8102.90 | 6778.92 |
| 6 layers | Electron | 0.14 | 0.17 | 5.44 | 5.48 | 311.08 | 309.89 | 10379.64 | 8391.39 |
| 7 layers | Electron | 0.14 | 0.17 | 5.59 | 5.77 | 360.24 | 359.21 | 11383.52 | 8773.73 |
| 8 layers | Electron | 0.14 | 0.17 | 5.50 | 5.19 | 415.22 | 413.09 | 13553.80 | 12470.88 |
| 9 layers | Electron | 0.14 | 0.16 | 5.93 | 5.83 | 467.41 | 466.37 | 13528.86 | 12220.08 |
| 10 layers | Electron | 0.14 | 0.16 | 5.54 | 5.79 | 518.14 | 516.62 | 17183.05 | 13724.44 |

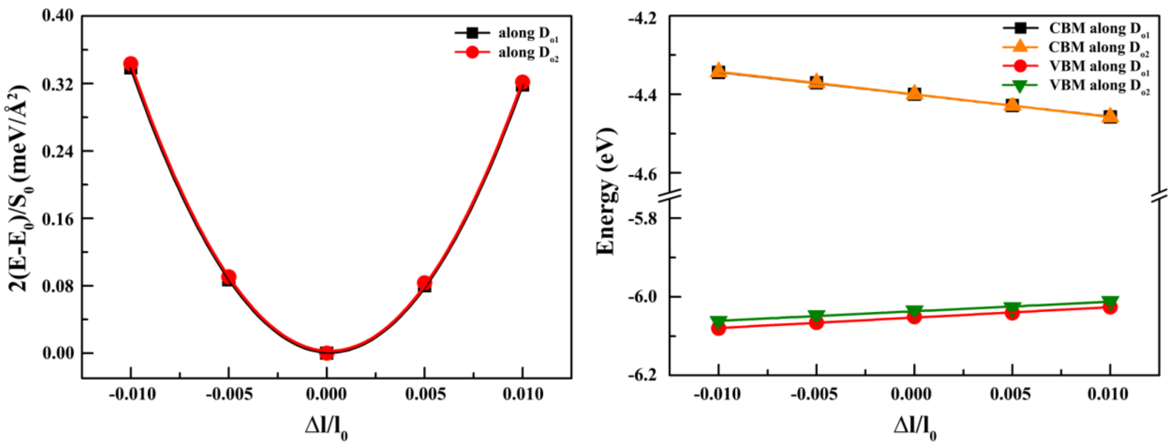


**Fig. S8** The 2D elastic modulus is obtained by fitting the strain energy density curves $2(E-E_0)/S_0$ versus $\Delta l/l_0$ for shared monolayer InSe. The strain is applied along the $D_{o1}$ and $D_{o2}$ directions.

## References


1 S. A. Semiletov, *Sov. Phys. Crystallogr. Krist.*, 1958, **3**, 292–297.

2 G. W. Mudd, S. A. Svatek, T. Ren, A. Patane, O. Makarovsky, L. Eaves, P. H. Beton, Z. D. Kovalyuk, G. V. Lashkarev, Z. R. Kudrynskyi and A. I. Dmitriev, *Adv. Mater.*, 2013, **25**, 5714–8.

3 R. Beardsley, A. V. Akimov, J. D. G. Greener, G. W. Mudd, S. Sandeep, Z. R. Kudrynskyi, Z. D. Kovalyuk, A. Patanè and A. J. Kent, *Sci. Rep.*, 2016, **6**, 26970.
